# Supplementary material for: The quasi-free-standing nature of graphene on H-saturated SiC(0001)
Source: arXiv:1103.3997 source file (2011-09-05)
Supplement: Supplementary file 1 [file supplemental.pdf]

# Supplementary information

## Evaluation of strain in graphene from Raman spectra

In an effort to estimate the strain present in our graphene samples, we make use of data published previously by Hanfland *et al.* [1] and Proctor *et al.* [2]. Hanfland *et al.* [1] measured the change of the lattice constant of graphite under hydrostatic pressure $P$ by means of x-ray diffraction. The in-plane lattice parameter $a$ was found to depend basically linearly on $P$ for the pressure range studied. Taking the data of Fig. 1 from Ref. [1], we find the following relationship:

$$\frac{\Delta a}{a_0} = -8 \times 10^{-4}\ \mathrm{GPa}^{-1} \cdot P, \tag{1}$$

where $a_0$ denotes the lattice constant at zero pressure. Furthermore, Hanfland *et al.* [1] measured Raman spectra of graphite under pressure. For increasing pressure, the Raman G line position shifts to higher wavenumbers as shown in Fig. 6 of Ref. [1]. In the pressure range below $\approx$ 6 GPa, we made a linear approximation of the relationship between G line position and pressure, yielding

$$\Delta_{G,\mathrm{strain}} = 4.4\ \mathrm{cm}^{-1}\ \mathrm{GPa}^{-1} \cdot P. \tag{2}$$

Combining relations (1) and (2), we obtain the dependence of the Raman G line position on the change of the in-plane lattice constant

$$\frac{\Delta a}{a_0} = -\frac{\Delta_{G,\mathrm{strain}}}{5.5\ \mathrm{cm}^{-1}} \times 10^{-3}. \tag{3}$$

In our evaluation of strain in our samples, we assume that this relation also holds for graphene and for tensile strain.

Proctor *et al.* [2] present data for the shift of the Raman G and 2D line in monolayer graphene on silicon as a function of hydrostatic pressure. (Note that for a thin layer of graphene bound to a thick substrate, the compression of the graphene is determined by the compression of the substrate. This results in different ranges of externally applied pressure for the same range of G line shifts for graphite and graphene on silicon, respectively. See Ref. [2] for details.)
For pressures below $\approx$ 2 GPa, we obtain a blueshift of $\Delta_{G,\mathrm{strain}} = 18.6\ \mathrm{cm}^{-1}/\mathrm{GPa}$ for the G line, whereas the 2D line shifts with a coefficient of $\Delta_{2D,\mathrm{strain}} = 38.3\ \mathrm{cm}^{-1}/\mathrm{GPa}$.

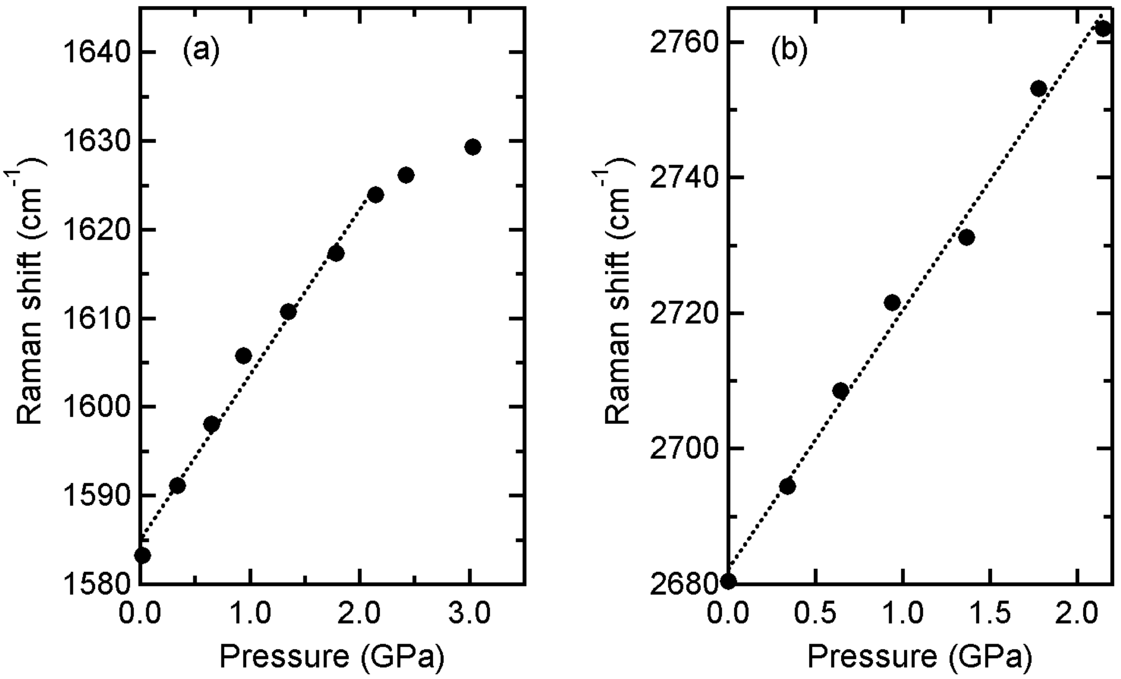


Figure 1: Change of the position of the Raman G line (a) and 2D line (b) for monolayer graphene on silicon. Data were taken from Ref. [2]. For $P$ below $\approx 2$ GPa, the G line position changes with a slope of 18.6 $\mathrm{cm}^{-1}$/GPa, whereas the 2D line position changes with a slope of 38.3 $\mathrm{cm}^{-1}$/GPa as indicated by the dotted lines.

Note that in both cases we used a linear approximation. Hence, the upshift of the 2D line position for a given pressure is larger than the shift of the G line by a factor of $\Delta_{2D,\mathrm{strain}}/\Delta_{G,\mathrm{strain}} = 2.1$. Finally, we combine this result with Eq. (3) to estimate the strain in our samples based on the 2D shift:

$$\frac{\Delta a}{a_0} = -\frac{\Delta_{2D,\mathrm{strain}}}{11.3\ \mathrm{cm}^{-1}} \times 10^{-3}. \tag{4}$$

## References


[1] M. Hanfland, H. Beister, K. Syassen, Phys. Rev. B **39**, 12598 (1989).

[2] J. E. Proctor, E. Gregoryanz, K. S. Novoselov, M. Lotya, J. N. Coleman, M. P. Halsall, Phys. Rev. B **80**, 073408 (2009).
